# Supplementary material for: Division Strategies Determine Growth and Viability of Growing-Dividing Autocatalytic Systems
Source: arXiv:2510.05675 ancillary file (2025-11-20)
Supplement: Supplementary file 1 [file SM.pdf]

# SUPPORTING INFORMATION

**Title of paper**: Division Strategies Determine Growth and Viability of Growing-Dividing Autocatalytic Systems
**Authors**: Parth Pratim Pandey and Sanjay Jain

## S1. The Hinshelwood 2-cycle: General derivations

The Hinshelwood 2-cycle (1) can be written in matrix form:

$$\begin{bmatrix} \dot{X}(t) \\ \dot{Y}(t) \end{bmatrix} = \begin{bmatrix} 0 & k_1 \\ k_2 & 0 \end{bmatrix} \begin{bmatrix} X(t) \\ Y(t) \end{bmatrix} = J \begin{bmatrix} X(t) \\ Y(t) \end{bmatrix}.$$

$J$ has two eigenvalues, $\lambda = \lambda_+ = \sqrt{k_1 k_2}$ and $\lambda_- = -\lambda$. The eigenvector for $\lambda_+$ is column vector $v_+ = [\sqrt{k_1} \quad \sqrt{k_2}]^T$ and for $\lambda_-$ it is $v_- = [\sqrt{k_1} \quad -\sqrt{k_2}]^T$. Any initial condition $z_0 = (X_0, Y_0) = [X_0 \quad Y_0]^T$ can be written as a column vector $z_0 = a_1 v_+ + a_2 v_-$ (where $a_1$ and $a_2$ depend on the initial conditions (ICs). Thus we can write the general solution $z(t) = e^{Jt} z_0 = a_1 e^{Jt} v_+ + a_2 e^{Jt} v_-$. This becomes:

$$\begin{bmatrix} X(t) \\ Y(t) \end{bmatrix} = a_1 e^{\lambda t} \begin{bmatrix} \sqrt{k_1} \\ \sqrt{k_2} \end{bmatrix} + a_2 e^{-\lambda t} \begin{bmatrix} \sqrt{k_1} \\ -\sqrt{k_2} \end{bmatrix}.$$

From the above matrix equation we get $X(t) = \sqrt{k_1}(a_1 e^{\lambda t} + a_2 e^{-\lambda t})$, $Y(t) = \sqrt{k_2}(a_1 e^{\lambda t} - a_2 e^{-\lambda t})$. Hence, indefinite growth (i.e., growth without any division) will drive the system to the attractor $Y = (\sqrt{k_2/k_1})X$. This line, which has slope $m_A = \sqrt{k_2/k_1}$), is in the direction of the vector $v_+$ in the XY plane, and will be referred to as the *asymptotic growth trajectory* (AGT).

Using methods developed in [12, 16], we will analytically solve for the growth-division trajectories when the above system undergoes repeated growth and division and discuss their stability. We first identify that the growth trajectories of this system are the hyperbolae in the XY plane:

$$X^2/k_1 - Y^2/k_2 = 4a_1 a_2. \tag{S1}$$

Thus in the growth phase of any generation the quantity $k_2 X^2 - k_1 Y^2$ will remain a constant. Considering this quantity at the beginning and at the end of the $g^{th}$ generation (the time interval between $t_g$ and $t_{g+1}$), we get *the constant of motion* in the $g^{th}$ generation,

$$k_2 X_g^2 - k_1 Y_g^2 = k_2 (X_g^M)^2 - k_1 (Y_g^M)^2, \tag{S2}$$

where $(X_g, Y_g) \equiv z_g$ denotes the *daughter state* at the beginning of the $g^{th}$ generation and $(X_g^M, Y_g^M) \equiv z_g^M$ denotes the *mother state* at the end of that generation just before division. In deriving (S2) from (S1) it is assumed that $z_g$ lies in the growth region.

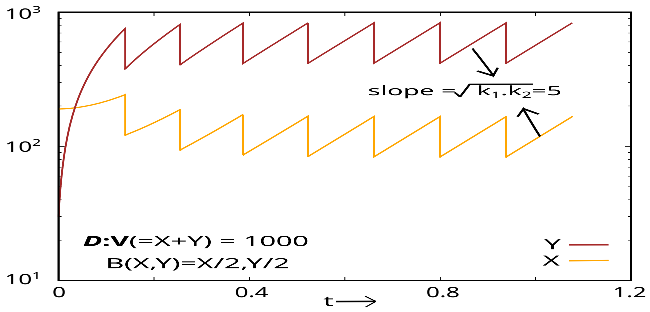


FIG. S1: Exponential growth of populations in the GDSS cycle for the 2-cycle undergoing GDD with $D = V$, $d = 1000$ with a standard birth map. Volume $V$ is defined as $V = X + Y$.

## S2. Balanced growth condition in the Hinshelwood cycle with standard birth map

In this section we prove that for the Hinshelwood cycle (Eq. (1)) following GDD with a standard birth map, if the division surface $S_D$ (defined by relation $D(X,Y) = d$) is such that it intersects the AGT only once transversally (not tangentially) at a finite point in the plane (excluding the origin and infinity), and the image of this point under the birth map is in the growth region, then the point of intersection defines a stable GDSS.

The last caveat in the above claim is needed because while the equation $D(X,Y) = d$ defines $S_D$, it does not specify which side of $S_D$ the growth and division regions are. Our convention is that the growth region corresponds to $D(X,Y) < d$. (Note that the division variable $D'(X,Y) = 1/D(X,Y)$ with threshold $d' = 1/d$ would give rise to the same division surface as $D(X,Y) = d$, but the growth regions for $D$ and $D'$ would be mutually exclusive.)

In Fig. 1d, the division variable is $D = X$ (with $d = 200$) with the standard birth map, $B(X,Y) = (X/2, Y/2)$. Notice that the division surface $S_D$ for $D \equiv X = d$ intersects the AGT of the Hinshelwood cycle (which is $Y = \sqrt{k_2/k_1 X}$) transversally at a non-trivial point. The case shown in Fig. 1e is another such example. It should be noted that many other choices of $D$ will also lead to a similar situation; i.e., its $S_D$ transversally intersects the AGT of the system (1). Some examples are $D = Y$, $D = X + Y$, $D = X^{\alpha_1} Y^{\alpha_2}$ with $\alpha_1 + \alpha_2 > 0$.

The GDD is defined by the division control variable $D(X,Y)$ and its threshold $d$. We denote a point in $\Gamma$ as $z = (X,Y)$. A general division surface ($S_D$) is $D(z) = D(X,Y) = d$ which defines a curve in the 2-dimensional phase space $\Gamma$. In general, for nonlinear functions $D(X,Y)$, the set of points satisfying $D(X,Y) = d$ can have multiple branches. We assume that only one of those branches is physical where division takes place.

In other words, $S_D$ is just a single curve in $\Gamma$, not a union of curves. When $D(X,Y)$ is independent of $Y$, this means that the division surface has the equation $X = a$ where $a$ is constant. When $D(X,Y)$ has a nontrivial dependence on $Y$, we can solve the equation $D(X,Y) = d$ for $Y$ in terms of $X$, obtaining the single valued function $h$ such that $Y = h(X)$. This is just the equation of the curve that defines $S_D$.

Under GDD, trajectories starting in the growth region shuttle from $S_B$ to $S_D$ and back to $S_B$ after the first division. Therefore, GDD defines a discrete time map $\mathcal{G}$ from $S_B$ to $S_B$ that maps the state of the daughter-at-birth in one generation to the state of the daughter-at-birth in the next generation, $z_{g+1} = \mathcal{G}(z_g)$. Therefore a GDSS, a limit cycle of GDD, corresponds to a fixed point $z^*$ of $\mathcal{G}$, $z^* = \mathcal{G}(z^*)$. If the GDSS limit cycle is a stable attractor of GDD, then $z^*$ is a stable fixed point of $\mathcal{G}$, and vice versa. Therefore in order to prove the stability of a GDSS we only have to prove that the corresponding $z^*$ is a stable fixed point of $\mathcal{G}$. In the case of the Hinshelwood 2-cycle, since $S_B$ is a 1-dimensional curve, the proof of stability of $\mathcal{G}$ reduces to the stability of a 1-dimensional discrete time map from the non-negative real line to itself, which we will denote $\mathcal{M}$.

We first prove the claim in the first para of this section for the simpler case when the division surface has the equation $X = a$. Then, since the standard birth map halves $X$ and $Y$, we have $X_g = X^M_{g-1}/2 = a/2$, $X^M_g = a$ and $Y^M_g = 2Y_{g+1}$. Substituting these values in Eq. (S2) gives

$$k_2(\frac{a}{2})^2 - k_1 Y_g^2 = k_2 a^2 - k_1(2Y_{g+1})^2, \tag{S3}$$

or

$$k_1(2Y_{g+1})^2 = k_1 Y_g^2 + \frac{3}{4}k_2 a^2. \tag{S4}$$

Eq. (S4) defines a one-dimensional discrete map $\mathcal{M}$ determining $Y_{g+1}$ in terms of $Y_g$, $Y_{g+1} = \mathcal{M}(Y_g)$. The fixed point of $\mathcal{M}$, where $Y_{g+1} = Y_g = Y^*$, is

$$Y^* = \sqrt{\frac{k_2}{k_1}}\frac{a}{2}. \tag{S5}$$

This defines the fixed point $z^* = (a/2, Y^*)$ of $\mathcal{G}$. Note that $z^*$ lies on the AGT. Therefore the growth trajectory of the daughter-at-birth that starts from $z^*$ remains on the AGT and ends where the division surface meets the AGT at $2z^*$. In Figs. 1d,e, $z^*$ is denoted by $z_\infty$.

To prove that $z^*$ is a stable fixed point of $\mathcal{G}$ we only need to prove that $Y^*$ is a stable fixed point of $\mathcal{M}$. The latter can be seen by evaluating the Jacobian of the map $\mathcal{M}$ at $Y^*$. Differentiating both sides of (S4) with respect to $Y_g$, we get

$$J(Y_g) = \frac{\partial \mathcal{M}(Y_g)}{\partial Y_g} = \frac{1}{4}\frac{Y_g}{Y_{g+1}}. \tag{S6}$$

Hence $J(Y^*) = 1/4$. Since the magnitude of the Jacobian of the map $\mathcal{M}$ evaluated at its fixed point is less than unity, $Y^*$ is a stable fixed point of $\mathcal{M}$. Hence $z^*$ is a stable fixed point of $\mathcal{G}$, and hence the GDSS limit cycle $z^*, 2z^*, z^*$ is a stable attractor of the GDD.

Now consider the general case of a division variable $D(X,Y)$ depending non-trivially on $Y$, such that the division surface $D(X,Y) = d$ is represented by the curve whose equation $Y = h(X)$. Using $\mathcal{A}_2$ we have $X_{g+1} = X^M_g/2$ and $Y_{g+1} = Y^M_g/2$. Thus

$$k_2 X_g^2 - k_1 Y_g^2 = k_2(2X_{g+1})^2 - k_1(2Y_{g+1})^2. \tag{S7}$$

Since the point $z^M_g = (X^M_g, Y^M_g)$ is on $S_D$, we have $Y^M_g = h(X^M_g)$ or $2Y_{g+1} = h(2X_{g+1})$. Similarly, since the point $z^M_{g-1} = (X^M_{g-1}, Y^M_{g-1})$ is also on $S_D$, we have $Y^M_{g-1} = h(X^M_{g-1})$ or $2Y_g = h(2X_g)$. Substituting $Y_g = h(2X_g)/2$ and $Y_{g+1} = h(2X_{g+1})/2$ in the above relation, we get

$$k_2 X_g^2 - \frac{k_1}{4}\Big(h(2X_g)\Big)^2 = 4k_2(X_{g+1})^2 - k_1\Big(h(2X_{g+1})\Big)^2. \tag{S8}$$

This equation defines the maps $\mathcal{M}$ and $\mathcal{G}$ as follows: Given a point $z_g = (X_g, Y_g)$ on $S_B$, (S8) implicitly finds $X_{g+1}$ which we denote as $X_{g+1} = \mathcal{M}(X_g)$. Then $Y_{g+1} = \frac{1}{2}h(2X_{g+1})$.

At a fixed point denoted by $z^* = (X^*, Y^*)$ of $\mathcal{G}$, we have $X_g = X_{g+1} = X^*$. Substituting this in (S8), we get

$$k_2(X^*)^2 - \frac{k_1}{4}(h(2X^*))^2 = 4k_2(X^*)^2 - k_1(h(2X^*))^2.$$

The solution of this equation satisfies

$$X^* = \frac{1}{2}\left(\sqrt{\frac{k_1}{k_2}}\right)h(2X^*). \tag{S9}$$

Since $X, Y$ are chemical populations, we consider only the positive solution.

(S9) implies that GDSS lies on the AGT. Since the mother-at-division is always on $S_D$, and in the GDSS its coordinates are $(2X^*, 2Y^*)$, we have $2Y^* = h(2X^*)$. Substituting this in (S9) gives $X^* = \sqrt{k_1/k_2}Y^*$, which implies that $(X^*, Y^*)$ is on the AGT. Since the AGT is a straight line passing through the origin, $(2X^*, 2Y^*)$ also lies on the AGT. In other words, the mother-at-division is at the point where $S_D$ meets the AGT, and the daughter-at-birth is where $S_B$ meets the AGT. We further know that a growth trajectory that starts on the AGT remains on the AGT, hence the entire GDSS lies on the AGT and is characterized by exponential balanced growth.

*Stability of the GDSS:* Since $X_{g+1} = \mathcal{M}(X_g)$, the Jacobian of the map $\mathcal{M}$ is given by $J(X_g) = \frac{d\mathcal{M}(X_g)}{dX_g}$. For stability of the GDSS we need the condition $|J(X^*)| < 1$.

Differentiating $X_{g+1}$ w.r.t. $X_g$ in Eq. (S8) and simplifying, we get

$$4\left[2k_2X_{g+1} - k_1h(2X_{g+1})\frac{dh(2X_{g+1})}{d(2X_{g+1})}\right]J(X_g) = \left[2k_2X_g - k_1h(2X_g)\frac{dh(2X_g)}{d(2X_g)}\right] \quad \text{(S10)}$$

At the fixed point, since $X_g = X_{g+1} = X^*$, the values of the expressions in the box brackets on both sides of Eq. (S10) are equal to each other. Whenever this value is nonzero and finite, we can conclude that

$$J(X^*) = 1/4$$

and hence for all such cases we have proved the GDSS is stable. The proof fails when the value of the expression in the box bracket at the fixed point either vanishes or becomes infinite. It is easy to see that this happens only in the following three cases.

(i) The division surface $Y = h(X)$ meets the AGT tangentially and not transversally at a nonzero finite point $z^*$ in the plane. Then the box bracket has the value $2k_2X^*(1 - \frac{m_{DS}}{m_A})$, where $m_{DS} = \frac{dh(u)}{du}\Big|_{u=2X^*}$ is the slope of the division surface at the point it meets the AGT, and $m_A = \sqrt{\frac{k_2}{k_1}} = \frac{h(2X^*)}{2X^*}$ is the slope of the AGT. This becomes zero if $S_D$ meets the AGT tangentially ($m_{DS} = m_A$) and the proof fails.
(ii) $S_D$ intersects the AGT at $X = 0$. Then again the box bracket on both sides of (S10) vanishes and the proof fails.
(iii) $S_D$ intersects the AGT at infinity. Then the terms in the box bracket on both sides of (S10) are infinite and again the proof fails.

## S3. Generalization to other linear dynamics

One can ask: What are the kinds of flows (defined by the general chemical population rate equations $dX_i/dt \equiv \dot{X}_i = f_i(X)$) for which a non-trivial stable GDSS will exist in such generality under the standard birth map? Based on the above example we conjecture that for linear systems (for which $f_i(X) = \sum_{j=1}^{N} c_{ij}X_j$ with $c_{ij}$ constant) a sufficient condition for the existence of a stable GDSS is that (a) the largest eigenvalue $\lambda_1$ of the matrix $C = (c_{ij})$ is positive, (b) the corresponding eigenvector (which defines the direction of the AGT) has all its components positive (in order for all $N$ chemical species to survive in the GDSS) and (c) the division variable $D(X)$ and its threshold $d$ are such that the division surface $D(X) = d$ transversally intersects the line from the origin along the direction of this eigenvector at a nonzero finite point in the physical phase space, and that the image of this point under the standard birth map is in the growth region $D(X) < d$.

## S4. Balanced growth condition in Hinshelwood cycle with a non-standard birth map

In this section we obtain the steady-state value $z_\infty$ for the Hinshelwood cycle (Eq. (1)), following GDD with $D(X, Y) = X$ and threshold $d$ and a non-standard birth map $B(X, Y) = (r, Y/2)$. This case is shown in Figs. 1c,f. In the constant of motion (Eq. S2) we substitute $X_g = X_{g+1} = r$, $X_g^M = d$, and $Y_g^M = 2Y_{g+1}$, thus obtaining the relation between $Y_g$ and $Y_{g+1}$:

$$Y_{g+1}^2 = \frac{k_1Y_g^2 + k_2(d^2 - r^2)}{4k_1}. \quad \text{(S11)}$$

We denote the above relation as $Y_{g+1} = \mathcal{M}(Y_g)$. At the fixed point of the map $\mathcal{M}$, $Y^{g+1} = Y^g = Y^*$. Substituting this in (S11), we get:

$$Y^* = \sqrt{\frac{k_2(d^2 - r^2)}{3k_1}}. \quad \text{(S12)}$$

This expression provides the coordinates of the point $z_\infty = (r, Y^*)$ in Fig. 1f, and hence the constants $a_1$ and $a_2$ in the equation of the hyperbola (S1) that represents the limit cycle trajectory in Fig. 1f.

It is easy to see that the Jacobian of the map $\mathcal{M}$, i.e., $J(Y_g) = \frac{d\mathcal{M}(Y_g)}{dY_g}$ computed at $Y_g = Y^*$ is $|J(Y^*)| = \left|\frac{d\mathcal{M}(Y_g)}{dY_g}(Y^*)\right| = 1/4$. Since $|J(Y^*)| < 1$, $Y^*$ is a stable fixed point of $\mathcal{M}$; hence this GDSS is stable.

**Ensuring total conservation of mass**:
The non-standard birth map used above, $B(X, Y) = (r, Y/2)$, leads to a violation of mass conservation in the following way: Consider the Hinshelwood cycle (Eq. (1)), following GDD with $D = X$, division threshold $d$, and a non-standard birth map $B(X, Y) = (r, Y/2)$. In the standard birth map, each daughter-at-birth would have got $X = d/2$. The resetting of $X$ to $r$ instead of $d/2$ is motivated by the observation that a certain amount of $X$ is lost after triggering division. In other words, $r < d/2$. The mother cell just before division has total chemical population $= d + Y$, whereas the total chemical population right after division (in the two daughter cells) is $2r + Y$. Thus a total population of $(d + Y) - (2r + Y) = d - 2r$ is unaccounted for, or lost. Biochemically, resetting a chemical population to a lower value would mean the conversion of that chemical into other chemicals, which would result in the simultaneous increase in their populations. In the Hinshelwood cycle the only population other than $X$ is $Y$. In order to conserve mass in the Hinshelwood cycle at the division step, one can assume that the population of $X$ getting lost due to resetting is added to the $Y$ population (assuming that the two molecules have the same mass). In other words,

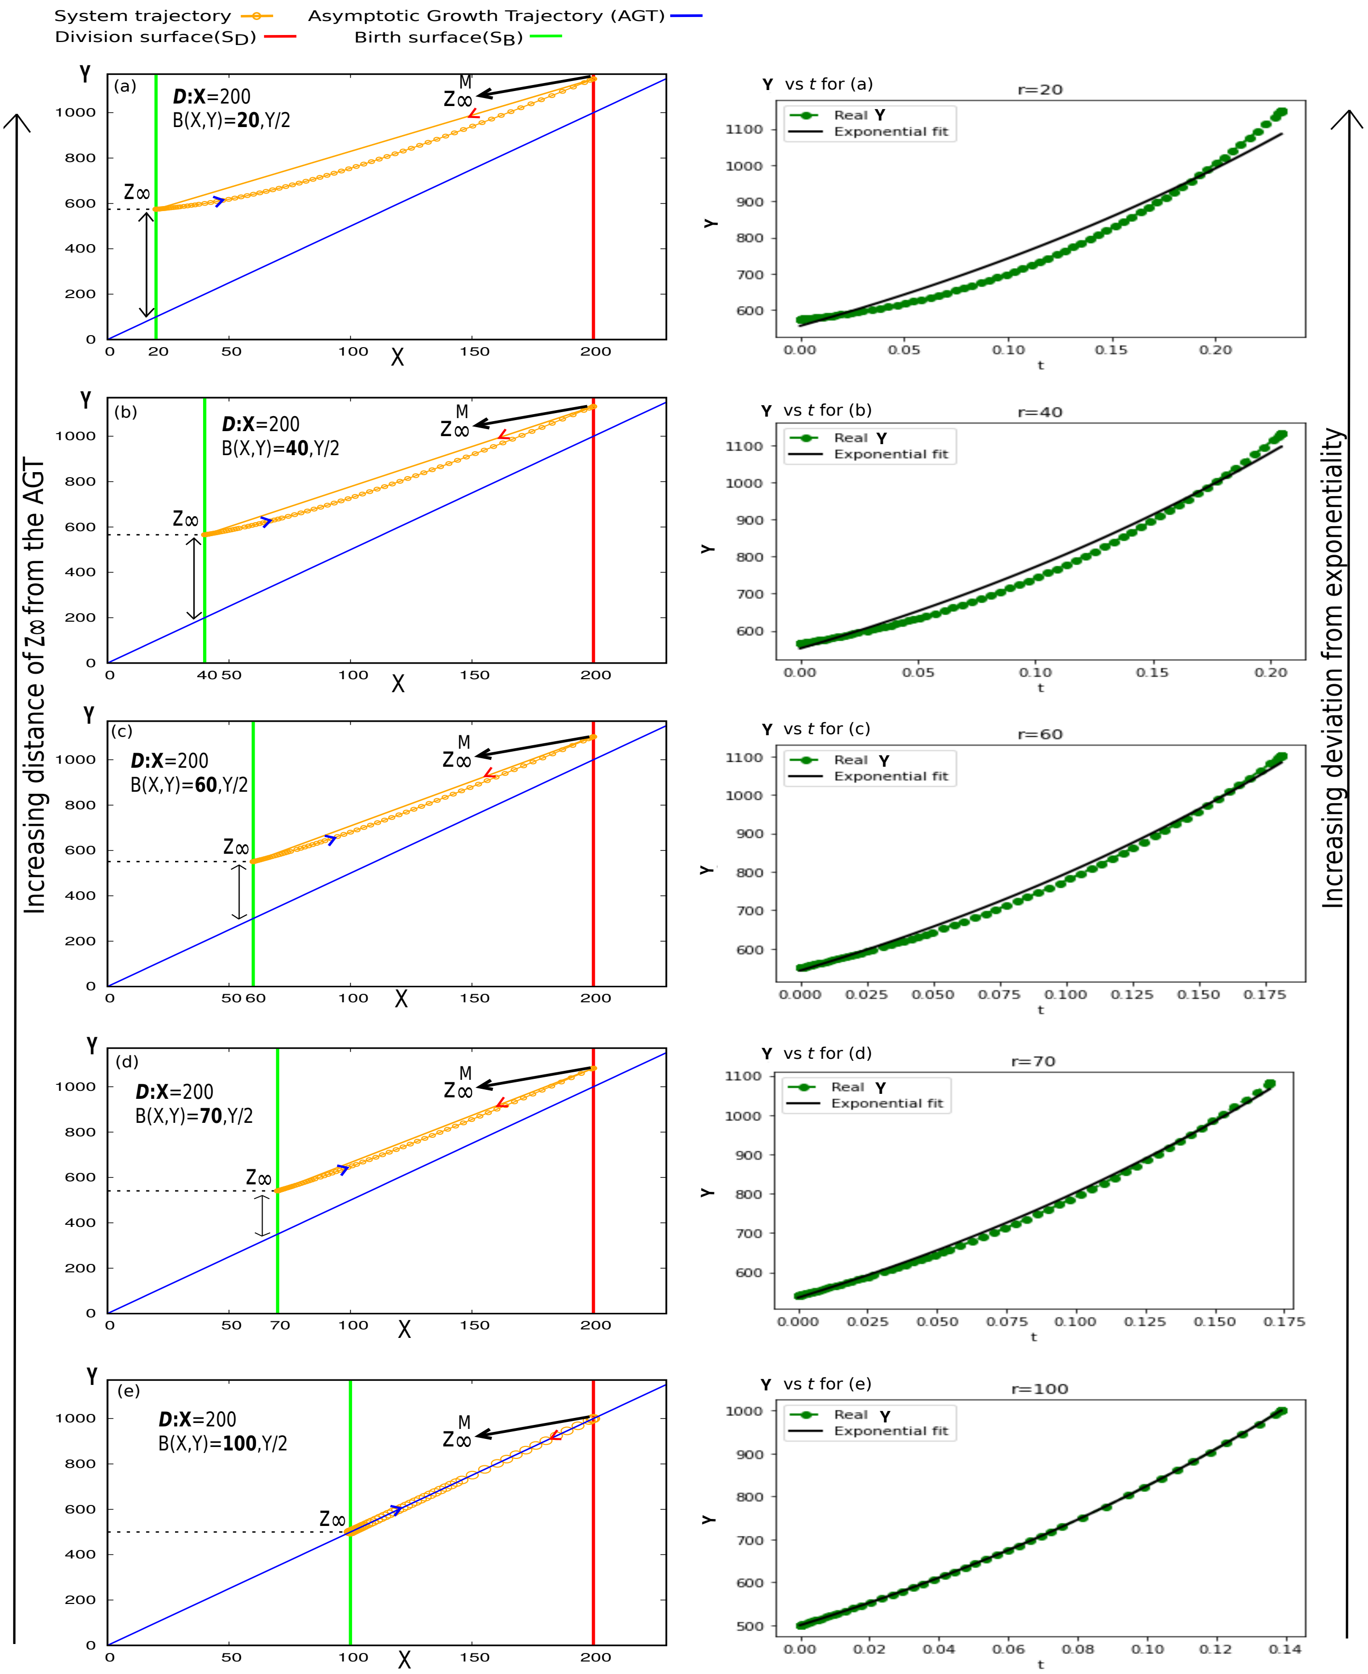


FIG. S2: Deviations from exponentiality in the Hinshelwood 2-cycle (Eq. (1)) undergoing GDD with a non-standard birth map. It is evident that as the birth map moves gradually from non-standard towards the standard birth map (by progressively changing $r$ from $< d/2$ to $d/2$ in the figures), the departure from exponentiality declines.

the instantaneous resetting of $X$ to a value $r < d/2$ at division is accompanied by the instantaneous conversion of a certain amount of $X$ into $Y$.

Thus, to ensure mass conservation one can use the birth map $B(X,Y) = (r, Y/2 + d/2 - r)$. I.e., while $X$ is reset to $r$ in the daughter cell, the population of $Y$ is not halved but is an amount $(d/2 - r)$ greater than half. Since there are two daughter cells, the extra amount of $2 \times (d/2 - r) = (d - 2r)$ is added to the total $Y$ pool, which is exactly the amount of $X$ that is being lost. Below we show that the Hinshelwood cycle (Eq. (1)) following GDD with $D = X$ (with threshold $d$), and with the modified non-standard birth map $B(X,Y) = (r, Y/2+d/2-r)$ (that ensures mass conservation in the sense described above) reaches a stable GDSS.

In the constant of motion (Eq. S2) we substitute $X_g = r$ and $X_g^M = d$, and using the relation $Y_{g+1} = Y_g^M/2 + d/2 - r$ we substitute $Y_g^M = 2(Y_{g+1} - d/2 + r)$. This yields

$$k_1(2Y_{g+1} - d + 2r)^2 = k_1 Y_g^2 + k_2(d^2 - r^2). \qquad \text{(S13)}$$

The above is a relation between $Y_{g+1}$ and $Y_g$ and can be rearranged as $Y_{g+1} = \mathcal{M}(Y_g)$. At the fixed point of the map $\mathcal{M}$, $Y_{g+1} = Y_g = Y^*$. Substituting this into Eq. (S13), we get:

$$(2Y^* - d + 2r)^2 = (Y^*)^2 + \frac{k_2}{k_1}(d^2 - r^2). \qquad \text{(S14)}$$

To analyze the stability of $Y^*$ we differentiate Eq. S13 w.r.t. $y_g$ and obtain:

$$\frac{dY_{g+1}}{dY_g} = \frac{Y_g}{2(2Y_{g+1} - d + 2r)}, \qquad \text{(S15)}$$

which is the Jacobian of the map $\mathcal{M}$, i.e., $J(Y_g) = \frac{d\mathcal{M}(Y_g)}{dY_g}$. Computing the Jacobian at the fixed point $Y_g = Y_{g+1} = Y^*$, we obtain:

$$J(Y_g = Y_{g+1} = Y^*) = \frac{1}{2}\left[\frac{Y^*}{(2Y^* - d + 2r)}\right]. \qquad \text{(S16)}$$

Now the factor in the box bracket is less than unity. This follows from the fixed point equation (S14), which implies that $2Y^* - d + 2r = [(Y^*)^2 + \frac{k_2}{k_1}(d^2 - r^2)]^{1/2} > Y^*$, because $r < d$. Therefore $J(Y^*) < 1$, which implies that the GDSS is stable.

We thus have shown that the GDD on the Hinshelwood cycle using a non-standard birth map that adheres to conservation of mass also generates a stable GDSS. Therefore the system exhibits balanced growth. The growth is non-exponential because the limit cycle (in particular the point $(r, Y^*)$) does not lie on the AGT.

## S5. Unbalanced growth for division processes with intensive division variables and a non-standard birth map

In this section we analytically show that for $D = X/V$ (with $V = X+Y$), with division threshold $d$, and the non-standard birth map $B(X,Y) = (r, Y/2)$, i.e., resetting $X$ at division, the Hinshelwood 2-cycle (1) can never have a stable GDSS.

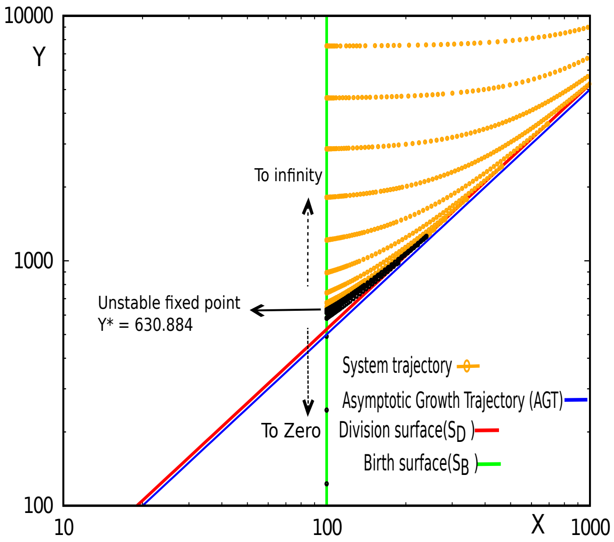


FIG. S3: Hinshelwood cycle (Eq. (1)) with $D = X/V$, $d = 0.16$ and the non-standard birth map $B(X,Y) = (100, Y/2)$ will either blow up to infinity or shrink to zero, depending upon the initial conditions. As shown in section S5, if $m_A < m_D < M_{max}$, then the fixed point (Eq. (S19)) is real but unstable. The parameters used in this figure are the same as in Fig. 2b for which this inequality holds. The value of the unstable fixed point is $Y^* \approx 630.884$ (as annotated in the figure). Two trajectories are shown in the figure, one with initial condition slightly above $Y^*$ (in orange), and another slightly below $Y^*$ (in black). It can be seen that the orange trajectory blows up to infinity whereas the black trajectory keeps shrinking until the system finds itself below the $S_D$ (i.e. in the 'division region') whereupon the system keeps dividing and ultimately dies ($Y$ becomes zero).

We first argue that for the current system with $D = X/(X+Y)$ and the non-standard birth map $B(X,Y) = (r, Y/2)$, it is essential that the slope of $S_D$ should be greater than the slope of the AGT. Since $D$ is $X/(X+Y) = d$, growth region is $X/(X+Y) < d$ or $Y/X > (1-d)/d$, i.e., the region **above** the line $Y = m_D X$ (where $m_D = (1-d)/d$). $S_D$ is $Y = m_D X$. It is thus geometrically obvious that if $S_D$ lies below AGT (that is, if $m_D < m_A$) then any trajectory starting in the growth region will never be able to divide because it will aymptotically converge towards the AGT and hence never hit the $S_D$ (see Fig. S4). The system will keep growing to infinity without ever dividing. This is also true if $m_D = m_A$. Thus for the system to experience growth-division cycles, the line $S_D$ should lie above AGT. i.e.,

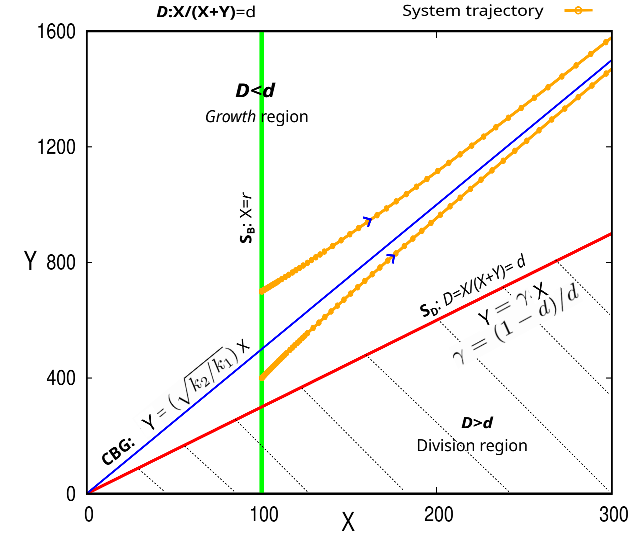


FIG. S4: For the case $D = X/V$ and $B(X, Y) = (r, Y/2)$, if the slope of $S_D$ (red line) is less than that of the AGT (blue line), then the system (1) tends to infinity since no trajectory in the growth region will be able to intersect the $S_D$, and hence the system will approach the AGT at infinity. Parameters: $k_1 = 1, k_2 = 25, d = 0.25$

$$m_D > \sqrt{k_2/k_1}. \tag{S17}$$

We now solve for the fixed point of the dynamics on $S_B$. Since $S_D$ is $Y = m_D X$, therefore $(X_g^M, Y_g^M)$ will satisfy $Y_g^M = m_D X_g^M$. And since the birth map is $B(X, Y) = (r, Y/2))$, hence $S_B$ is the surface $X = r$. Therefore $X_{g+1} = r$ and $Y_{g+1} = Y_g^M/2$ for all generations $g$.

We now substitute the three previously obtained relations, $X_g = X_{g+1} = r$, $Y_{g+1} = Y_g^M/2$, and $Y_g^M = m_D X_g^M$ into the constant of motion equation (S2), and by simplification we get

$$Y_{g+1}^2 = \frac{m_D^2(k_1 Y_g^2 - k_2 r^2)}{4(k_1 m_D^2 - k_2)}. \tag{S18}$$

Therefore, given a point $z_g = (r, Y_g)$ on $S_B$, (S18) implicitly finds $z_{g+1} = (r, Y_{g+1})$. (S18) gives us the map $\mathcal{M}$ which is defined by $Y_{g+1} = \mathcal{M}(Y_g)$.

Let us denote the fixed point of $\mathcal{M}$ by $Y^*$. Substituting $Y_g = Y_{g+1} = Y^*$ in (S18), we get:

$$Y^* = \sqrt{\frac{k_2 r^2 m_D^2}{(4k_2 - 3k_1 m_D^2)}}. \tag{S19}$$

From Eq. (S19) we find that for $Y^*$ to be real the parameters need to satisfy the condition

$$m_D < m_{max}, \tag{S20}$$

where $m_{max} \equiv \left(\frac{4k_2}{3k_1}\right)^{\frac{1}{2}} = \frac{2}{\sqrt{3}} m_A$.

Combining the two conditions (S17) and (S20), we obtain

$$m_A < m_D < m_{max}. \tag{S21}$$

The above arguments show that if and only if the system satisfies the condition (S21), a periodic GDSS trajectory exists. However it turns out that this periodic GDSS trajectory is unstable.

To show that we now obtain the condition for the stability of the fixed point given by (S19). Since $Y_{g+1} = \mathcal{M}(Y_g)$, the Jacobian of the transformation is given by $J(Y_g) = \frac{d\mathcal{M}(Y_g)}{dY_g}$. For stability of the fixed point $Y^*$ we need the condition $|J(Y^*)| = \left|\frac{d\mathcal{M}(Y_g)}{dY_g}(Y^*)\right| < 1$.

Differentiating $Y_{g+1}$ w.r.t. $Y_g$ in Eq. (S18) and evaluating it at $Y^*$, we get

$$\frac{d\mathcal{M}(Y_g)}{dY_g}(Y^*) = \frac{1}{4\left(1 - \frac{m_A^2}{m_D^2}\right)}.$$

Hence the condition for stability of $Y^*$ becomes

$$\left|\frac{1}{\left(1 - \frac{m_A^2}{m_D^2}\right)}\right| < 4, \tag{S22}$$

The above modulus function can be simplified in the following two ways: If we assume $1 - (m_A^2/m_D^2) > 0$ and substitute it in (S22), then we get $m_D^2 > 4k_2/3k_1$ which clearly violates condition (S21) obtained above. The other option is to assume $1 - (m_A^2/k_1 m_D^2) < 0$. But this straight away means $m_D < m_A$ which again violates the condition (S21).

Hence we have shown that condition (S21) and (S22) can not be satisfied simultaneously which implies that for $D = X/V$ and birth map $B(X, Y) = (r, Y/2)$ we can never obtain a real, non-trivial GDSS which is stable.

Accepting the fact that the GDSS can never be stable in this case, one can still ask what happens to the growing-dividing system. Condition (S21) hints that the parameter space is generically divided into three cases: (i) $m_D > m_{max}$, (ii) $m_A < m_D < m_{max}$, and (iii) $m_D < m_A$.

[Case (i)]: $m_D > m_{max} \implies (1-d)/d > (2/\sqrt{3})\sqrt{k_2/k_1}$, which implies $d < \sqrt{3k_1}/(\sqrt{3k_1} + \sqrt{4k_2}$. For $k_1 = 1, k_2 = 25$, this inequality becomes $d < 0.1476$. Below we show that for this case, regardless of the initial condition, $Y$ always approaches zero (a simulation with $d = 0.14$ is shown in Fig. 2a).

One can simplify the map Eq. (S18) to:

$$Y_{g+1}{}^2 = \frac{Y_g^2 - (k_2 r^2/k_1)}{4\big(1 - k_2/(k_1 m_D^2)\big)}.$$

$$= \frac{Y_g^2}{4\big(1 - k_2/(k_1 m_D^2)\big)} - \frac{(k_2 r^2/k_1)}{4\big(1 - k_2/(k_1 m_D^2)\big)} \qquad \text{(S23)}$$

Since $m_D > (2/\sqrt{3})\sqrt{k_2/k_1}$, hence it is trivial to show that $4\big(1 - k_2/(k_1 m_D^2)\big) > 1$ and $\frac{(k_2 r^2/k_1)}{4\left(1 - k_2/(k_1 m_D^2)\right)} > 0$. Since these two conditions are independent of the generation $g$, hence on applying these two conditions on the above map Eq. (S23) we obtain $Y_{g+1} < Y_g$. Thus one can say that starting from any initial condition $Y_0$, there exists a finite $g$ such that $Y_g$ becomes small enough for the point $z_g = (r, Y_g)$ to enter into the division region. After that the system will keep dividing and ultimately $Y$ will go to zero. The same argument applies if $r = 0$.

[Case (ii)]: $m_{AGT} < m_D < (2/\sqrt{3})m_{AGT} \implies \sqrt{(k_2/k_1)} < (1-d)/d < (2/\sqrt{3})\sqrt{k_2/k_1}$, which implies $\sqrt{3k_1}/(\sqrt{3k_1} + \sqrt{4k_2} < d < \sqrt{k_1}/(\sqrt{k_1} + \sqrt{k_2})$. For $k_1 = 1, k_2 = 25$, this inequality becomes $0.1476 < d < 0.1667$. In this case there exists a real, non-trivial fixed point given by Eq. (S19), and hence there exists a periodic trajectory of the GDD. But this fixed point is unstable, as proven above. Thus, if the system starts above the fixed point, the growing-dividing system will blow up to infinity, and on starting below the fixed point it will converge to zero. In Fig. 2b we have shown the case for which the initial condition is above the unstable fixed point and hence after each division the system becomes larger and larger. In Fig. S3 we have shown both kinds of initial conditions for this case.

[Case (iii)]: $m_D < m_{AGT} \implies (1-d)/d < \sqrt{(k_2/k_1)}$, which implies $d > \sqrt{k_1}/(\sqrt{k_1} + \sqrt{k_2}) = 0.1667$ (for $k_1 = 1, k_2 = 25$). This has already been discussed in Fig. S4 ($d = 0.25$) where the $S_D$ lies below the AGT and hence a trajectory starting in the growth region never hits the $S_D$ and hence the system will keep growing without ever dividing.

### S6. Making intensive division variables work

In this section we present a strategy by which even an intensive division variable (such as a concentration) can lead to robust compositional homeostasis. We find that if the non-standard birth map is such that the variable reset at division is different from the chemical whose concentration is chosen to be the division variable, we can get a stable GDSS. For example, say the concentration of $X$ is chosen as the division variable for the Hinshelwood 2-cycle (Eq. (1)). Then, if the resetting variable in the non-standard birth map is $Y$, we will get a stable GDSS (in other words, the intensive division variable $D(X,Y) = X/V$ works if the birth map is chosen to be $B(X,Y) = (X/2, r)$). Similarly, the division variable $D(X,Y) = Y/V$ works if the birth map is chosen to be $B(X,Y) = (r, Y/2)$, i.e., if $X$ is reset at division.

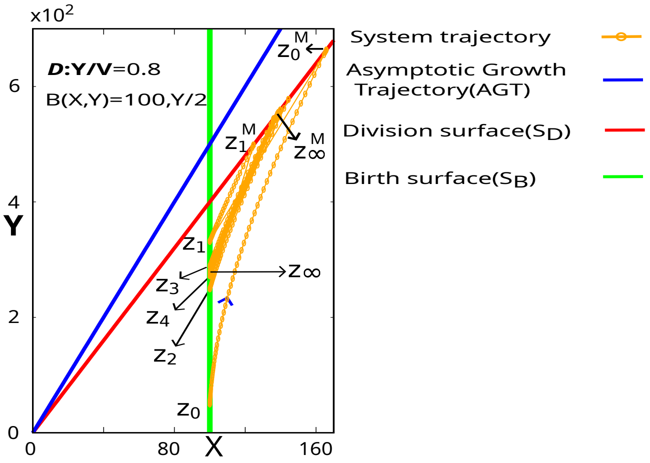


FIG. S5: Making intensive variables work by choosing an appropriate non-standard birth map. Balanced growth with the division variable as the concentration of $Y$, $D = Y/(X+Y)$ with $B(X,Y) = (100, Y/2)$, i.e., $X$ is reset at division. IC: $(X,Y) = (100, 180)$. Parameters: $k_1 = 1$, $k_2 = 25$, $d = 0.8$.

In Fig. S5, we show the Hinshelwood cycle (Eq. (1)) reaching a stable GDSS with an intensive variable as the division variable, here $D = Y/V$ where $V = X+Y$. Since $D$ is a 'concentration' type variable, as discussed above, we choose a non-standard birth map where the resetting variable is different from the one whose concentration is the division variable. Since the concentration of $Y$ is the division variable, hence we choose $X$ to be the resetting variable in the birth map, i.e., $B(X,Y) = (r, Y/2)$. Since $D = Y/(X+Y)$ with threshold $d$, the growth region is $Y/(X+Y) < d$ which simplifies to $Y/X < d/(1-d)$. Thus, $S_D$ is the line $Y = m_D X$ where $m_D = d/(1-d)$ (red line) and the *growth region* is the region *below* this line. $S_B$ is $X = 100$ (green line). Below we show that for this case, a stable non-trivial GDSS exists if $m_D < \frac{2}{\sqrt{5}} m_A$, which is equivalent to $d < \sqrt{4k_2}/\big(\sqrt{4k_2} + \sqrt{5k_1}\big)$. It can be seen that GDD drives the system to a GDSS that is not on the AGT (i.e., $z_\infty$ does *not* lie on the AGT (the blue line)). Thus $X$ and $Y$ will be deviated from exponential growth in the GDSS cycle.

As mentioned above, the growth region in this case is *below* $S_D$, hence it is geometrically obvious that slope of $S_D$ should be *smaller* than that of the AGT (i.e., $S_D$ should lie below the AGT) for any growth trajectory to hit the $S_D$. Fig S6 shows the case when the slope of $S_D$ is more than that of the AGT (i.e., $S_D$ lies above the AGT). It is apparent in the figure that for such a case all trajectories in the growth region never hit the $S_D$ and hence the system blows up to infinity without ever dividing. This provides us the first necessary condition

for this system to grow and divide, i.e., slope of $S_D <$ slope of AGT. I.e.,

$$m_D < m_A,$$
$$\implies m_D < \sqrt{k_2/k_1}. \tag{S24}$$

Further, we have $X_{g+1} = r$ and $Y_{g+1} = Y_g^M/2$ for all $g$. $S_B$ is the surface $X = r$. Since the mother cell at division has to be on the division surface, $(X_g^M, Y_g^M)$ satisfies $Y_g^M = m_D X_g^M$.

Substituting the above mentioned three relations, $X_{g+1} = r$, $Y_{g+1} = Y_g^M/2$, and $Y_g^M = \beta X_g^M$ in the constant of motion, Eq. S2, and simplifying it, we get a relation between $Y_{g+1}$ and $Y_g$:

$$Y_{g+1}^2 = \frac{m_D^2(k_1 Y_g^2 - k_2 r^2)}{4(k_1 m_D^2 - k_2)}. \tag{S25}$$

This equation defines the map $\mathcal{M}$ as follows: Given a point $z_g = (r, Y_g)$ on $S_B$, (S25) implicitly finds $Y_{g+1}$ which we denote as $Y_{g+1} = \mathcal{M}(Y_g)$. Substituting $Y_g = Y_{g+1} = Y^*$ in (S25) to find the fixed point of $\mathcal{M}$, we get

$$Y^* = \sqrt{\frac{k_2 r^2 m_D^2}{(4k_2 - 3k_1 m_D^2)}}. \tag{S26}$$

It is obvious that the condition

$$m_D^2 < \frac{4k_2}{3k_1} \tag{S27}$$

is necessary for $Y^*$ to be real.

Differentiating $Y_{g+1}$ w.r.t. $Y_g$ in Eq. (S25) and evaluating it at $Y^*$, we get

$$J(Y^*) = \frac{d\mathcal{M}(Y_g)}{dY_g}(y^*) = \frac{1}{4\left(1 - \dfrac{m_A^2}{m_D^2}\right)}.$$

Hence the condition for stability of $Y^*$, i.e., $|J(Y^*)| < 1$ becomes

$$\left|\frac{1}{\left(1 - \dfrac{m_A^2}{m_D^2}\right)}\right| < 4, \tag{S28}$$

Now condition (S24) tells us that $\left(1 - \dfrac{k_2}{k_1 m_D^2}\right) < 0$. Substituting this in the condition (S28), on simplification, we get:

$$m_D^2 < \frac{4k_2}{5k_1},$$
$$\implies m_D < \frac{2}{\sqrt{5}} m_A \tag{S29}$$

Notice that, unlike the case in section S5, here all the three conditions, i.e., (S24), (S27) and (S29) can be satisfied simultaneously.

Since condition (S29) is the strictest among the three conditions, we only need to satisfy this condition for the system (1) to have a stable, non-trivial GDSS with $D = Y/V$ and threshold $d$ and birth map $B(X,Y) = (r, Y/2)$. Since $m_D = d/(1-d)$, this condition is equivalent to $d < \sqrt{4k_2}/\left(\sqrt{4k_2} + \sqrt{5k_1}\right)$.

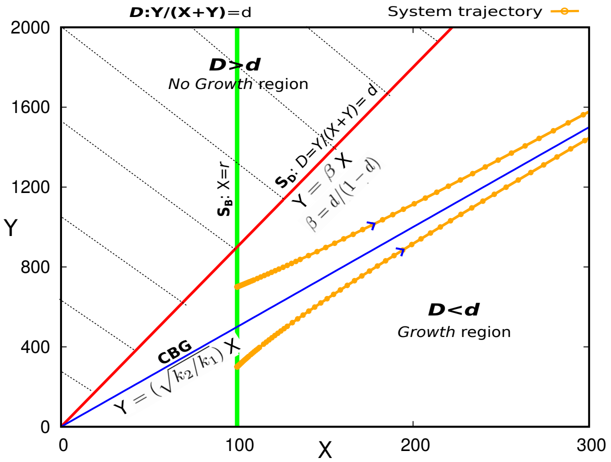


FIG. S6: For the case shown in Fig. S5, i.e., $D = Y/V$ and $B(X,Y) = (r, Y/2)$, if the slope of $S_D$ (red line) is greater than that of the AGT (blue line), then the system (1) tends to infinity since no trajectory in the growth region will be able to intersect the $S_D$, and hence the system will approach the AGT at infinity.

## S7. A nonlinear Precursor-Lipid-Catalyst ($PLC$) model of a protocell with GDD shows a behaviour similar to the Hinshelwood 2-cycle

The $PLC$ protocell model is similar to another coarse-grained model for bacteria [9, 44] and consists of 3 types of molecules; precursors ($P$), lipids ($L$) and catalysts ($C$). The protocell has the following 3 reactions: (i) $P_{ext} \xrightarrow{L} P$, (ii) $P \xrightarrow{C} L$, and (iii) $P \xrightarrow{C} C$. The first reaction transports an external precursor molecule through the lipid membrane into the interior of the protocell, while the second and third convert the precursor molecules in the interior of the protocell into lipid and catalyst molecules, respectively, both catalyzed by $C$. The $L$ molecules are assumed to migrate immediately upon formation to the cell boundary and constitute the surface of the cell. The bulk of the cell consists of $P$ and $C$ molecules, hence we assume that the instantaneous volume $V$ is a function of the molecular abundances of $P$ and $C$, i.e., $V = a(P+C)$. The growth dynamics of the $PLC$ protocell is based on well-stirred, non-linear mass-action chemical kinetics, de-

scribed by the following set of differential equations:

$$\frac{dP}{dt} = k_P L\bigg([P_{ext}] - \frac{P}{V}\bigg) - (k_L + k_C)\frac{CP}{V} - \phi_P P,, \tag{S30a}$$

$$\frac{dL}{dt} = k_L \frac{CP}{V} - \phi_L L,, \tag{S30b}$$

$$\frac{dC}{dt} = k_C \frac{CP}{V} - \phi_C C, \tag{S30c}$$

where $P$, $L$ and $C$ represent the *number* (not concentration) of the molecules. $[P_{ext}]$ is the concentration of $P_{ext}$ (assumed constant). The rate of $P$ transport inside the cell is proportional to the membrane area $S$ (where $S = bL$) as well as to the concentration difference $[P_{ext}] - (P/V)$ across the membrane. $k_L$ and $k_C$ are the rate constants at which $L$ and $C$ are produced from the consumption of $P$ via the catalytic action of $C$. $\phi_P$, $\phi_L$ and $\phi_C$ are the degradation rates of $P$, $L$ and $C$ molecules respectively into a waste product. Note that equations (S30) do not contain a term proportional to $\dot{V}/V$ on the right-hand side because they refer to abundances $X_i$ instead of concentrations $X_i/V$.

### *i. The PLC protocell exhibits an exponential GDSS, non-exponential GDSS or death depending upon the division mechanism*

We now show that the distinct behaviours observed in the growing-dividing linear Hinshelwood 2-cycle are analogously present in the generic cellular model, the *PLC* protocell. Firstly, the growing-dividing *PLC* protocell reaches an exponential GDSS with division control variables with degree $> 0$ and a standard birth map $B(P, L, C) = (P/2, L/2, C/2)$. Fig. S7 illustrates this for the following $D$ variables: (i) abundance of $P$, $L$, or $C$, (ii) volume (chosen as a linear function of chemical abundances), (iii) surface area $S$ (a linear function of the surface-chemicals $L$), (iv) reduced surface area $\frac{S}{S_0(V)}$ [26], a nonlinear function of abundances characterizing the departure of the shape of the protocell from a spherical shape. (Remark: Here $S$ is the surface area of the cell and $S_0(V) = (36\pi V^2)^{1/3}$ is the surface area of a sphere of volume $V$ where $V$ is volume of the cell. When $\frac{S}{S_0(V)} = 1$, $S = S_0(V)$ and the cell must be spherical. When $S > S_0(V)$, the cell must be a deformed sphere. At $\frac{S}{S_0(V)} = 2^{1/3}$, $S = 2S_0(V/2)$, *i.e.,* the surface area $S$ is large enough to form the boundary of two spherical cells of volume $V/2$ each. In the *PLC* protocell model, $S = bL$ and $V = a(P + C)$.)

Second, GDD with $D$ variables of degree $> 0$ but with a non-standard birth map lead to a non-exponential GDSS. E.g., Fig. S8 shows the protocell reaching a non-exponential GDSS with $D = C$ (with $d = 100$) and a non-standard birth map $B(P, L, C) = (P/2, L/2, r)$, i.e., at division the abundance of $C$ is reset to a predefined value $r$ ($r = 1$ in Fig. S8).

Third, just like the Hinshelwood cycle, the protocell dies (either blows up or shrinks to zero) if the $D$ variable is the concentration of a chemical species and the non-standard birth map is such that the abundance of the same chemical species (whose concentration was chosen as the $D$ variable) is reset in the non-standard birth map. E.g., $D = C/V$ and $B(P, L, C) = (P/2, L/2, r)$. Depending upon the value of $d$ (and the IC) the system either collapses to zero or expands to infinity (see Fig. S9a,b). Similar results were obtained for (i) $D = P/V$ and $B(P, L, C) = (r, L/2, C/2)$, and (ii) $D = L/V$ and $B(P, L, C) = (P/2, r, C/2)$).

Finally, we find that the strategy mentioned earlier to make concentration-type division variables work for the Hinshelwood cycle also works for the protocell. Fig S9c shows the protocell reaching a non-trivial GDSS with $D = P/V$ and with the non-standard birth map $B(P, L, C) = (P/2, L/2, r)$. I.e., the chemical whose concentration is the $D$ variable (here $P$) and the chemical whose abundance is reset at division (here $C$) are chosen to be different.

### *ii. The geometric similarity between the PLC protocell and the Hinshelwood 2-cycle*

In the previous subsection we provided numerical evidence that GDD of the *PLC* protocell exhibits the same kind of behaviour as the Hinshelwood 2-cycle. It would be useful to have a geometric or analytical understanding of this for the *PLC* protocell, just as we provided for the Hinshelwood 2-cycle. The nonlinearity of the *PLC* growth equations (S30) prevents us from providing derivations as explicit as for the Hinshelwood 2-cycle, which has linear growth equations (1). However, we show below analytically that the *PLC* model, like the Hinshelwood 2-cycle, has a line passing through the origin of its phase space, along which all three populations grow exponentially with the same growth rate. Further, we provide numerical evidence that this line is the attractor of the growth dynamics. This means that this line is the asymptotic growth trajectory (AGT) of the *PLC* model. In other words, the *PLC* model, though nonlinear, shares with the Hinshelwood 2-cycle the geometric property that its AGT is a straight line passing through the origin of its phase space, along which all populations exhibit exponential growth with the same rate.

Fig. S10a shows a trajectory of the *PLC* protocell (Eq. S30) when it is allowed to grow uninterrupted, without any division. (In other words Eq. S30 is simulated directly without imposing the division cutoff.) As can be seen from the common slope of the trajectories after an initial transient, all three populations, $P$, $L$ and $C$, end up growing exponentially with the same rate. This sug-

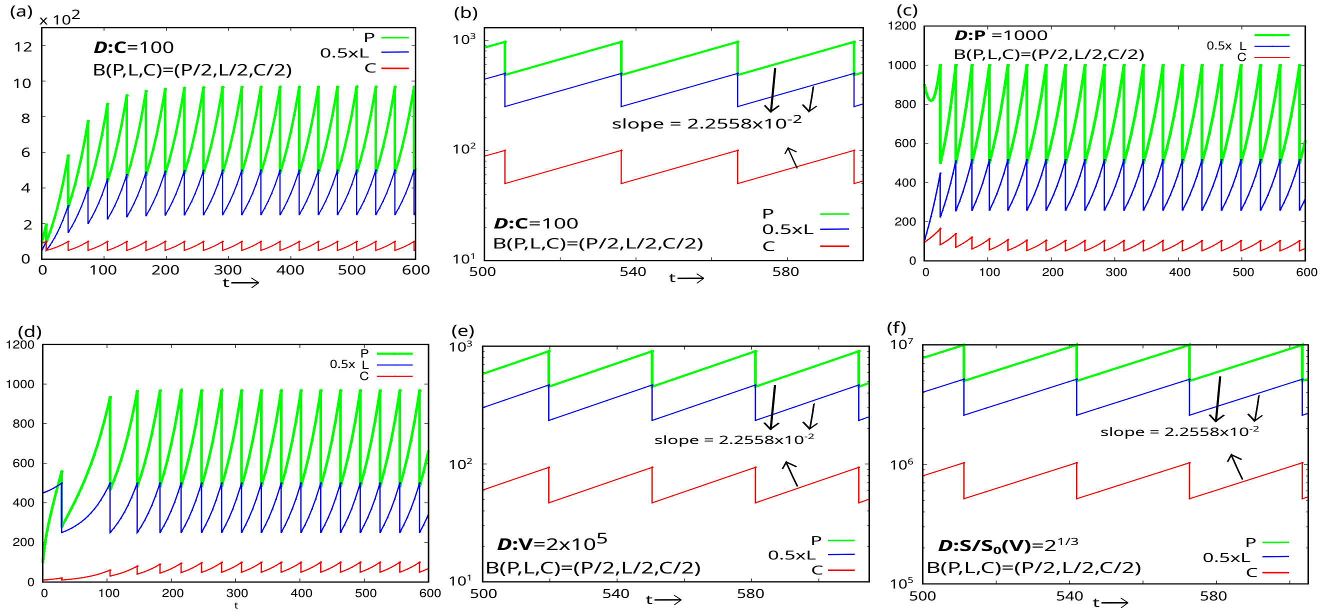


FIG. S7: The growing-dividing $PLC$ protocell exhibiting exponential balanced growth for several division variables with degree $> 0$ and the standard birth map. (a) Trajectory of the chemical abundances versus time for the *PLC protocell* implementing GDD with $D = C$, $d = 100$, and standard birth map $B(P, L, C) = (P/2, L/2, C/2)$. IC: $P_0 = L_0 = 100$, $C_0 = 90$. (b) The semi-log plot of (a) showing that all the trajectories become exponential with the same exponential growth rate as highlighted by the slopes. The value of the slope matches the growth rate theoretically calculated using the formula Eq. (S36). (c) GDSS with $D = P$, $d = 10^3$, IC: $P_0 = 900, L_0 = 200$, $C_0 = 95$ (d) GDSS with $D = L$, $d = 10^3$, IC: $P_0 = 100, L_0 = 900, C_0 = 10$ (e) GDSS with $D = V$, $d = 2 \times 10^5$, IC: $P_0 = 300, L_0 = 500$, $C_0 = 500$ and, (f) GDSS with $D = S/S_0(V)$, $d = 2^{1/3}$, IC:$P_0 = 10^7, L_0 = 7 \times 10^6, C_0 = 3 \times 10^6$. All are with a standard birth map $B(P, L, C) = (P/2, L/2, C/2)$. Parameters: $k_P = 100$, $k_L = 50$, $k_C = 5$, $[P_e] = 5 \times 10^{-3}$, $a = 1/[P_e]$, $b = 1$, $\phi_P = \phi_L = \phi_C = 10^{-4}$. $L$ has been scaled by factor of 0.5 as mentioned in the legends to enhance the clarity of the plots.

gests that we consider the ansatz

$$P(t) = P_0 e^{\mu t}, \quad L(t) = L_0 e^{\mu t}, \quad C(t) = C_0 e^{\mu t} \tag{S31}$$

as a possible solution of the equations (S30), where $P_0, L_0, C_0$ and $\mu$ are constants. Notice that under this ansatz ratios of the chemical populations ($C(t)/P(t)$, $C(t)/L(t)$ and $L(t)/P(t)$ are time independent constants. Since the protocell volume also grows as $e^{\mu t}$ under this ansatz, the concentrations are also constant in time. In phase space, this trajectory is a ray starting at the origin at $t = -\infty$, passing through the point $(P_0, L_0, C_0)$ at $t = 0$, and continuing in the same direction for $t > 0$ all the way to infinity if $\mu > 0$. (For $mu < 0$ the trajectory moves towards the origin along the same line.)

On substituting the ansatz Eq. (S31) in the protocell dynamics (S30) we find that in each of the three population rate equations, both sides become proportional to $e^{\mu t}$, and therefore $t$ cancels out from both sides, leading to the three algebraic equations:

$$\mu P_0 = k_P L_0 \left( [P_e] - \frac{P_0}{b(P_0 + C_0)} \right)$$
$$-(k_L + k_C) \frac{P_0 C_0}{b(P_0 + C_0)} - \phi_P P_0, \tag{S32a}$$

$$\mu L_0 = k_L \frac{P_0 C_0}{b(P_0 + C_0)} - \phi_L L_0, \tag{S32b}$$

$$\mu C_0 = k_C \frac{P_0 C_0}{b(P_0 + C_0)} - \phi_C C_0. \tag{S32c}$$

where $P_0, L_0, C_0$ and $\mu$ are as yet unknown.

Eqs. (S32b) and (S32c) fix the ratios of the chemicals in terms of the parameters of the model and $\mu$. Specifically from (S32c) we get (setting $\phi_P = \phi_L = \phi_C = \phi$ for convenience),

$$\frac{C_0}{P_0} = \frac{k_C/b - (\mu + \phi)}{\mu + \phi}, \tag{S33}$$

and from (S32b) and (S32c) together we get,

$$\frac{C_0}{L_0} = \frac{k_C}{k_L}. \tag{S34}$$

The equations (S33) and (S34) determine the direction of a 1-dimensional line passing through the origin in the 3-dimensional phase space of chemical populations $P$, $L$

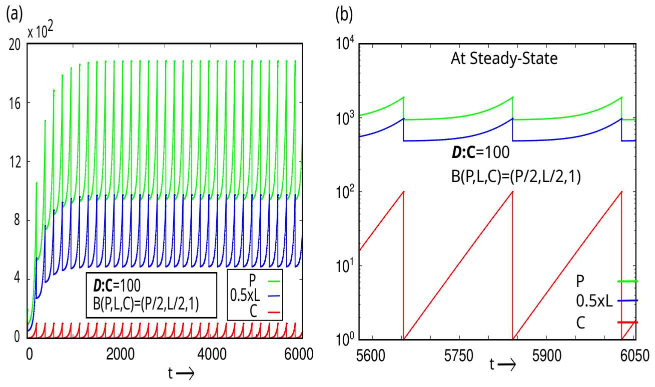


FIG. S8: The growing-dividing $PLC$ protocell exhibiting a non-exponential GDSS for $D$ with degree $> 0$ and a non-standard birth map. (a) The trajectory of the chemical abundances versus time for the $PLC$ protocell implementing GDD with $D = C$, $d = 100$ with a non-standard birth map $B(P, L, C) = (P/2, L/2, 1)$. IC: $P_0 = L_0 = 100$, $C_0 = 90$. (b) The semi-log plot of (a) showing that the $P$ and $L$ abundance do not become exponential with time. Parameters are same as in Fig. S7.

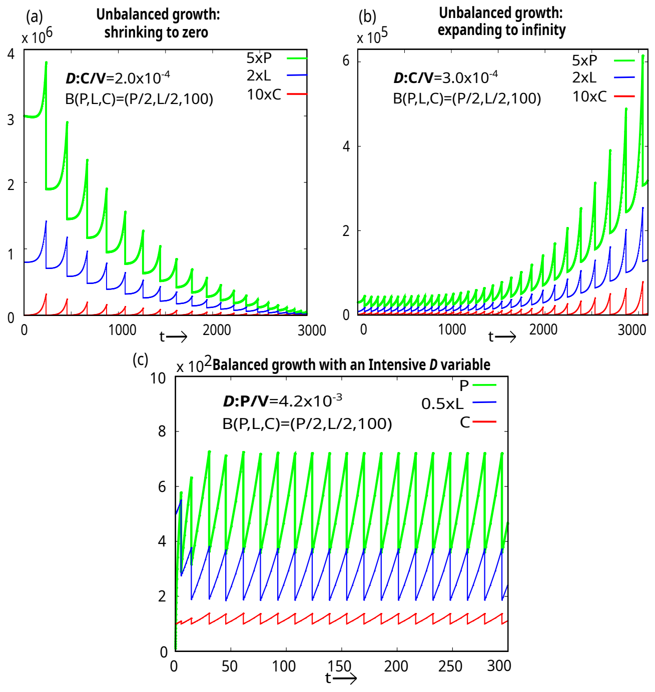


FIG. S9: PLC model with intensive $D$ variables: System death with one combination of $D$ variable and birth map, and balanced growth with another combination. In (a) the system progressively shrinks, and in (b) the system progressively grows larger after each division. In both cases the concentration of $C$ is chosen as the division variable, i.e., $D = C/V$, with $d = 2.0 \times 10^{-4}$ in (a), and $d = 3.0 \times 10^{-4}$ in (b). $D = C/V$ being an intensive variable, we choose a non-standard birth map $B(P, L, C) = (P/2, L/2, 100)$ (i.e., the abundance of $C$ is reset to 100 at division). (c) Balanced growth with concentration of $P$ as $D$, i.e., $D = P/V$, $d = 4.2 \times 10^{-3}$ and non-standard birth map $B(P, L, C) = (P/2, L/2, 100)$, i.e., $C$ is the variable reset at birth. The other parameters are same as in Fig. S7. $P$,$L$,$C$ have been scaled by factors indicated in the legends to enhance the clarity of the plots.

and $C$ (analogous to the AGT: $Y = (\sqrt{k_2/k_1})X$ for the Hinshelwood cycle). The third ratio $P_0/L_0$, the fractional composition of the cell and all steady state concentrations $\frac{P}{V}, \frac{L}{V}, \frac{C}{V}$ can be derived from (S33) and (S34) in terms of the parameters and the (as yet undetermined) growth rate $\mu$. To determine $\mu$, using (S33) and (S34) in (S32a) we can eliminate $P_0$, $L_0$ and $C_0$ from (S32a) and get the following quadratic equation in $\mu + \phi$:

$$\alpha(\mu + \phi)^2 - \beta(\mu + \phi) + \gamma = 0, \tag{S35}$$

where $\alpha, \beta, \gamma$ are the constants (all positive) given in terms of the parameters by

$$\alpha = \frac{k_L(k_C + k_P)}{k_C^2},$$
$$\beta = \left(\frac{k_P k_L\left([P_e] + 1/b\right)}{k_C} + \frac{(k_L + k_C)}{b}\right),$$
$$\gamma = \frac{k_P k_L [P_e]}{b}.$$

The above quadratic gives 2 solutions $\mu_\pm = \dfrac{\beta \pm \sqrt{\beta^2 - 4\alpha\gamma}}{2\alpha} - \phi$. Of these two solutions $\mu_+$ is unphysical, as substituting it in (S33) we find the ratio $C_0/P_0$ to be negative. Hence

$$\mu = \frac{\beta - \sqrt{\beta^2 - 4\alpha\gamma}}{2\alpha} - \phi. \tag{S36}$$

For fixed values of the parameters, Eq. (S33) and Eq. (S34) define a straight line passing through the origin in the 3-dimensional phase space $\Gamma$ (whose coordinate axes are $X_1 = P$, $X_2 = L$, $X_3 = C$). Therefore, the above analysis shows that an exponential solution (S31) exists if and only if the initial values $P_0, L_0, C_0$ lie on this line. If the system does lie on this line, the trajectory of all the chemical populations and the volume (since the latter is a linear function of the populations) will be exponential, all with the same rate given by Eq. (S36). Since ratios of the $X_i$ remain constant under the ansatz, the trajectory will stay on this line for all time.

Further, Figs. S10a,b suggest that this line (defined by Eq. (S33) and Eq. (S34)) is also the *attractor* of the system, i.e., after long times, the system trajectory in the 3-dimensional phase space converges to this line. We find numerically that for a wide range of initial conditions the slopes and ratios converge to the same values as in Figs. S10a,b. This pattern is repeated for other parameter values. Since the straight line defined by Eq. (S33) and Eq. (S34)) is the attractor of the $PLC$ growth dynamics (S30), this line is the Asymptotic Growth Trajectory (AGT) of the $PLC$ system.

Since the AGT is a straight line passing through the origin, it is invariant under the standard birth map. All the degree $> 0$ division variables considered in the previous subsection for the $PLC$ model cut this AGT transversally once in the finite region of the physical phase space.

This is probably the geometric reason for the existence of a stable GDSS for such division variables, with exponential growth when we use the standard birth map and non-exponential growth when we use a non-standard birth map. For concentration type division variables, the division surface is a plane passing through the origin. E.g., if $D(P, L, C) = C/V$, the division surface $D(P, L, C) = d$ is the plane with the equation $adP + (ad-1)C = 0$. This plane is invariant under the standard birth map, and it intersects the AGT line only at the origin, analogous to what happened in the Hinshelwood 2-cycle.

We suspect that this geometric similarity between the Hinshelwood 2-cycle and $PLC$ growth dynamics (namely the fact that both have AGTs that are straight lines passing through the origin) is behind the strikingly similar behaviour of the GDD in the two cases.

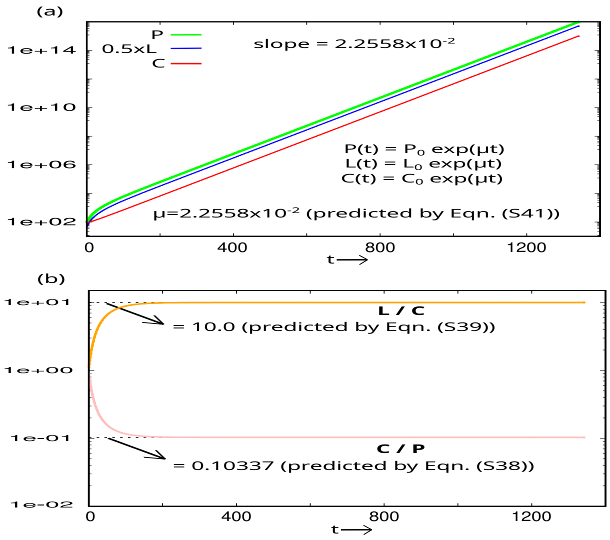


FIG. S10: Characteristics of the $PLC$ system when growing indefinitely (without division being imposed). (a) Semi-log plot of the chemical populations versus time for the $PLC$ protocell dynamics (Eq. (S30)). After a transient all the three populations grow exponentially with the same exponent (as shown by the identical slope of the trajectories). The slope obtained from simulations matches the predicted growth rate value obtained analytically in Eq. (S36). (b) This plot shows the chemical population ratios reaching constant values, which match perfectly with the analytically obtained values from Eq. (S33)) and Eq. (S34). Parameters and IC are the same as in Fig. S7.

The fact that both systems have an AGT that is a straight line passing through the origin is in turn a consequence of the fact that in both cases the functions $f_i$ defining the growth dynamics are homogeneous degree one functions of the $X_i$. These functions appear in the rate equations $dX_i/dt = f_i(X), \quad i = 1, 2, ..., N$. When they satisfy the homogeneous degree one scaling property ($f_i(\beta X) = \beta f_i(X)$ for all $i = 1, 2, ..., N$ and for all $\beta > 0$), as they do for the Hinshelwood 2-cycle and the $PLC$ growth dynamics (S30), the equations generically admit exponentially growing solutions for the populations (e.g., (S31) for the $PLC$ system), as was shown in reference [9]. Further the ratios of the populations in these solutions as well as the exponential growth rate are determined by the parameters appearing in the functions $f_i$. These ratios define a line passing through the origin of the phase space. In many cases such a solution is an attractor of the dynamics, thereby implying that an AGT of the system is a line passing through the origin of phase space. Reference [9] also showed that the above mentioned homogeneous degree one property of the $f_i$ is generically true for all growing chemical systems whose volume is itself a homogeneous degree one function of the chemical population. The volume being a linear function of the populations (such as in the $PLC$ protocell) is a special case of that property. This chain of arguments suggests that when the volume of a growing chemical system is a homogeneous degree one function of the populations within it, the AGT is quite generically a line passing through the origin. For such systems, the properties of the GDD discussed above are likely to hold.
